# Supplementary material for: Fast multifrequency measurement of nonlinear conductance
Source: arXiv:1809.07671 source file (2018-12-17)
Supplement: Supplementary file 1 [file suppmat.pdf]

# Supplemental material for "Fast multifrequency measurement of nonlinear conductance"

Riccardo Borgani,[1,*] Mojtaba Gilzad Kohan,[2] Alberto Vomiero,[2] and David B. Haviland[1]

[1]*Nanostructure Physics, KTH Royal Institute of Technology, 10691 Stockholm, Sweden*

[2]*Department of Engineering Sciences and Mathematics, Luleå University of Technology, 97187 Luleå, Sweden*

(Dated: 20 September 2018)

## INSTRUMENTATION

The current flowing through the AFM tip $I$ is converted to voltage by a variable-gain low-noise current amplifier DLPCA-200 (FEMTO Messtechnik GmbH). The voltage is then sampled by a digital multifrequency lock-in amplifier (MLA, Intermodulation Products AB), and the real and imaginary part of 32 frequency components $\{I_{\mathrm{G}k}\}$ and $\{I_{\mathrm{D}k}\}$ are read via ethernet by a computer for analysis. Two output ports on the MLA are used to apply the sample bias $V$ and the compensation voltage $V_{\mathrm{C}}$. The measurement and analysis routines are implemented in the scripting interface of the MLA control software. They are written in Python and make use of the inverse Fast Fourier Transform[1] and other routines in the SciPy and NumPy libraries[2].

The measurements on the organic solar cell sample are performed on a NanoWizard ULTRA Speed AFM (JPK Instruments AG) mounted on an inverted optical microscope (Nikon Corporation). The microscope objective is used to focus the light from a white light-emitting diode (LED) onto a small spot around the area scanned. The LED illumination is alternately switched on and off during the scanning trace and retrace ($\approx$ 1 Hz) in order to compare the electrical response of the material under light and dark conditions. The measurements on the $CuO_2$/ZnO sample are performed on a Dimension Icon AFM (Bruker Corporation). In both cases, the AFM is operated in contact mode with a RMN-12PT400B cantilever (Bruker, nominal spring constant 0.3 N/m).

In principle, the current amplifier built-in in the AFM can be used instead of the external DLPCA. However, the external amplifier used in this study allows for easier access to the input guard, and therefore for easier implementation of the compensation routine. Similarly one could perform the experiments described herein without the MLA, by using a high-speed sampling card synchronized with two signal generators. Care must be taken that all the frequencies of interest are tuned to minimize Fourier leakage, and the analysis would need to be performed entirely on the computer (limiting the real-time capabilities of the analysis).

## SYMMETRY OF IVC

An arbitrary curve can be decomposed into an even- and an odd-symmetry curve around zero. For our IVC:

$$I_{\mathrm{G}}(V) = I_{\mathrm{even}}(V) + I_{\mathrm{odd}}(V), \tag{S1}$$

$$I_{\mathrm{even}}(V) = \frac{1}{2}[I_{\mathrm{G}}(V) + I_{\mathrm{G}}(-V)], \tag{S2}$$

$$I_{\mathrm{odd}}(V) = \frac{1}{2}[I_{\mathrm{G}}(V) - I_{\mathrm{G}}(-V)]. \tag{S3}$$

We then quantify the magnitude of each contribution by using the norm

$$||I||^2 = \frac{1}{2V_{\mathrm{AC}}} \int_{-V_{\mathrm{AC}}}^{V_{\mathrm{AC}}} |I(V)|^2 \, \mathrm{d}V, \tag{S4}$$

and the symmetry parameter defined as

$$S = \frac{||I_{\mathrm{even}}||}{||I_{\mathrm{even}}|| + ||I_{\mathrm{odd}}||}. \tag{S5}$$

$S$ is equal to zero for a purely odd curve, equal to one for a purely even curve, and between zero and one for any other curve.

## MATERIAL PROPERTIES MAPPING ON ORGANIC PHOTOVOLTAIC MATERIAL

Figure S1 shows a comparison of the current measured on the organic photo-voltaic material under illumination and in dark conditions. The displacement current (green line), and thus the capacitance are not affected by the change in illumination. The galvanic current, on the other hand, significantly decreases in dark conditions: the diode-like shape of the IVC disappears together with $I_{\mathrm{SC}}$ and $V_{\mathrm{OC}}$, and only a high residual resistance is visible.

Figure S2 shows the reconstructed values of $I_{\mathrm{SC}}$, $V_{\mathrm{OC}}$ and the current $I_{\mathrm{RV}}$ measured at a reverse bias of 1 V. Due to the computational efficiency of the iFFT, the analysis of the entire scan takes less than one second on a notebook computer and can therefore be performed in real time, while scanning with the AFM. In all the panels showing current (**a**, **c** and **d**), a vertical line and an horizontal line are visible on the left and at the bottom, respectively. These low-current features are indication of damage to the sample material caused by a previous scan with too high contact-mode setpoint.

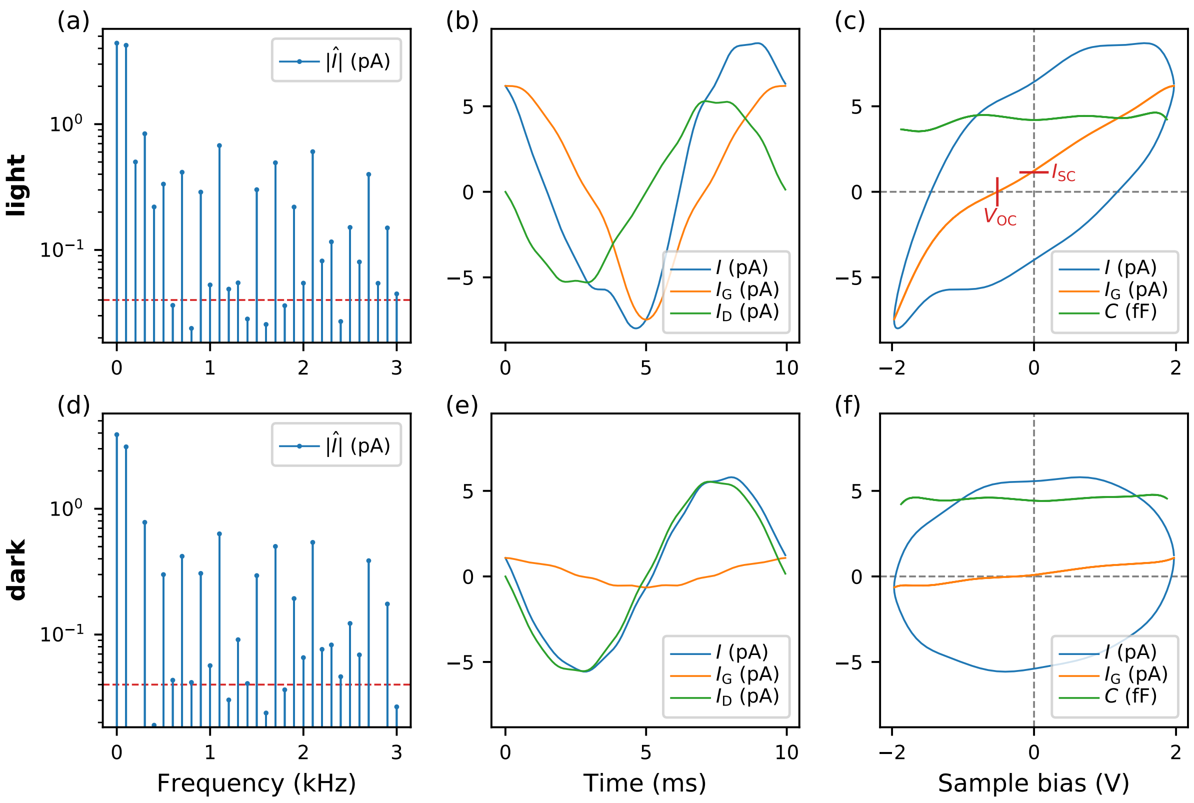


FIG. S1. **Current-voltage characteristics on a photo-active polymer blend.** Measurement under light (a-c) and dark (d-f) conditions. (a) and (d), amplitude of the measured current at 31 frequencies, the phase is also measured but not shown. The red dashed line is the calibrated noise level. (b) and (e), total, galvanic and displacement currents as a function of time obtained from the current spectrum by inverse Fourier transform of Eq. (5) in the main text. (c) and (f), reconstructed currents and junction capacitance vs. voltage. The loop in the total current $I(V)$ is due to the junction capacitance. The galvanic current $I_G(V)$ does not show such a loop. The junction capacitance $C$ is nearly constant, as expected. Panels (a)-(c) are reproduced in Fig. 2 in the main text.

## HEIGHT IMAGES

Figure S3 shows the AFM height images obtained from the quasistatic mode (contact mode) feedback, *i.e.* at constant cantilever deflection.

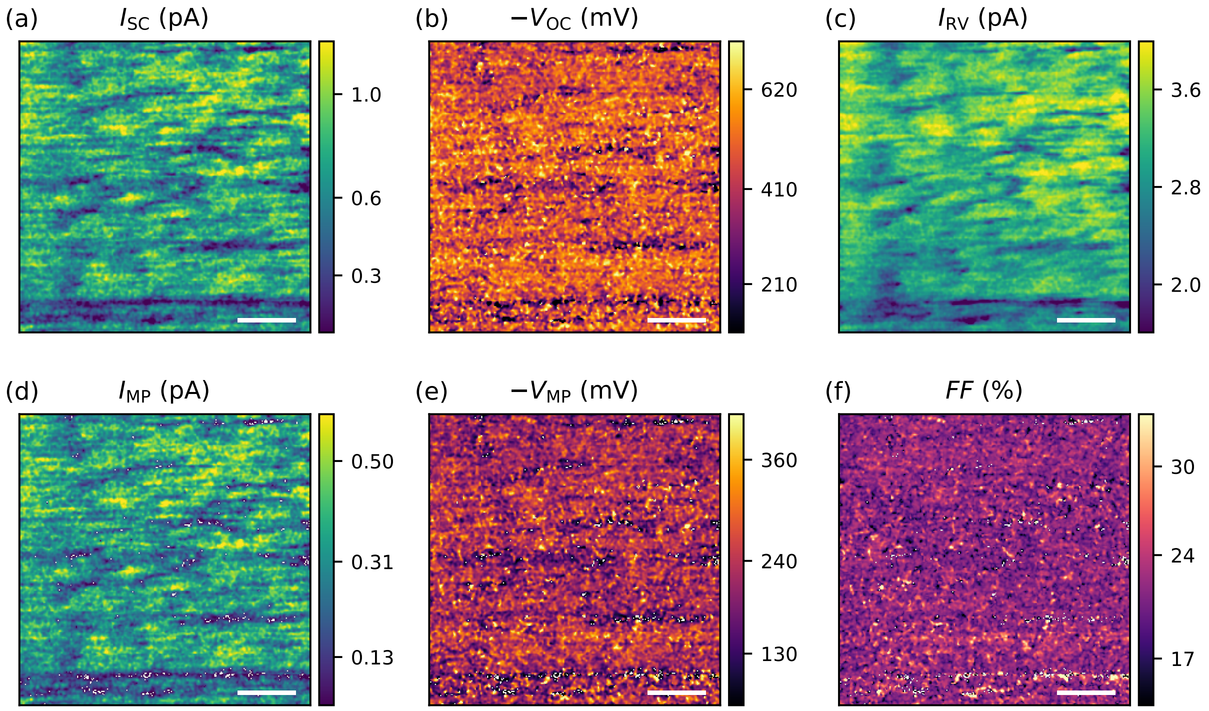


FIG. S2. **Parameter maps on a photo-active polymer blend.** Maps and histograms of: (a) short-circuit current $I_{\mathrm{SC}}$; (b) open-circuit voltage $V_{\mathrm{OC}}$; (c) reverse-bias current $I_{\mathrm{RV}}$; (d) current at maximum-power point $I_{\mathrm{MP}}$; (e) voltage at maximum-power point $V_{\mathrm{MP}}$; (f) fill factor $FF = (I_{\mathrm{MP}}V_{\mathrm{MP}})/(I_{\mathrm{SC}}V_{\mathrm{OC}})$. The white scale bars are 200 nm.

* borgani@kth.se

[1] J. W. Cooley and J. W. Tukey, Mathematics of Computation **19**, 297 (1965).

[2] E. Jones, T. Oliphant, P. Peterson, *et al.*, "SciPy: Open source scientific tools for Python," (2001–), [online, available at http://www.scipy.org/].

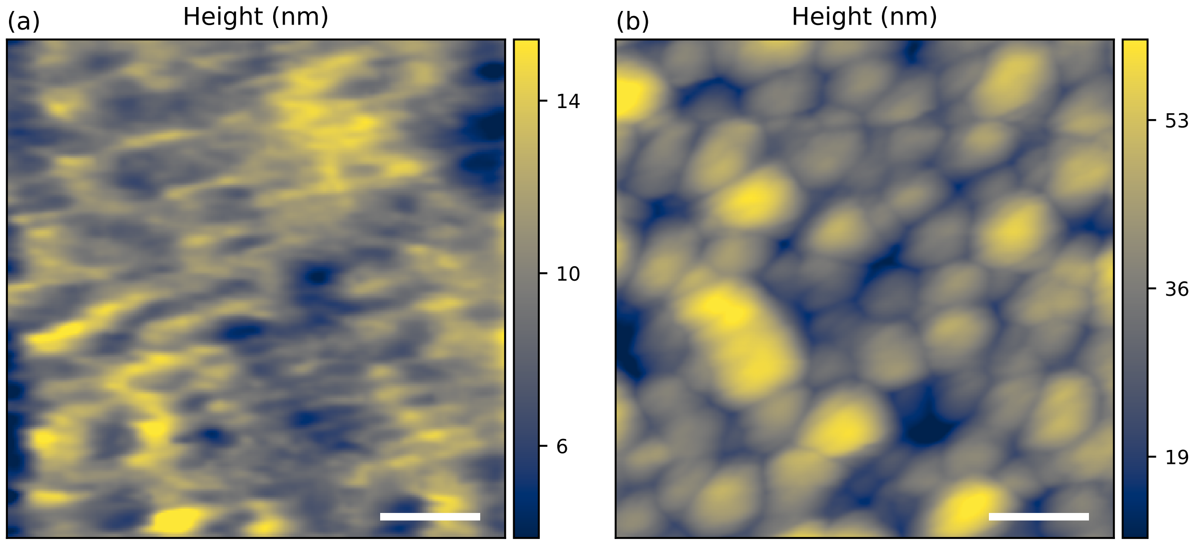


FIG. S3. **Height images.** (a) organic photovoltaic material of Fig. S2 and Fig. 2 in the main text. (b) thin-film all-oxide p/n junction of Fig. 3 in the main text. The white scale bars are 200 nm.
